# Supplementary material for: Making Auctions Robust to Aftermarkets
Source: arXiv:2107.05853 source file (2022-11-16)
Supplement: Supplementary file 1 [file invest.tex]

\section{Investment Incentives}
\label{apx:invest}

In this section, we first show that the welfare benchmark introduced in \cref{sec:invest intro} may not be attainable given any mechanism under equilibrium. 
Recall that this benchmark considers the best investment \emph{profile} in hindsight.
 
\begin{example}\label{exp:benchmark}
There are two agents. The types of the agents are drawn independently, each drawn uniformly from $\{\type_1,\type_2\}$. 
For any type in $\{\type_1,\type_2\}$, if the agent does not invest (cost of 0) then she has a value of $0$. 
If an agent of type $\type_1$ invests, bearing a cost of $3$, her value becomes $5$, while  
if an agent of type $\type_2$ invests, bearing a cost of $2$, her value becomes $10$.

As the investment decision of each agent is only based on her private type, an agent of type $\type_1$ needs to decide if to invest not knowing the type of the other. If both agents have type $\type_1$ and none of them invest, the welfare is 0, lower than the benchmark defined in \cref{sec:invest intro}. If both invest, one of them incurs a cost not incurred by the benchmark.  
If only one of them invests, her investment cost is incurred even when the other has type $\type_2$, a case in which only the other should invest to obtain the benchmark. 
Therefore, even if the mechanism maximizes welfare for the realized investment decisions, it cannot maximize welfare ex ante (as some investment decisions are sub optimal).  
\end{example}

%\mbc{OLD version of the example (to be removed after the above is approved):}
%\begin{example}\label{exp:benchmark}
%	There are two agents. 
%	Both agents have two types $\{\type_1,\type_2\}$ drawn from independent uniform distributions. 
%	For type $\type_1$, the agent can choose to not invest with value~$0$, 
%	or invest with value $5$ and cost $3$. 
%	For type $\type_2$, the agent can choose to not invest with value~$0$, 
%	or invest with value $10$ and cost $2$. 
%	
%	To attain the welfare benchmark in \cref{sec:invest intro}, 
%	both agents with type $\type_1$ cannot invest because otherwise with probability $\sfrac{1}{2}$, 
%	the opponent will have a different type $\type_2$ and investment leads to an additional cost of $3$ compared to the benchmark. 
%	Note that for any mechanism, 
%	the investment decision of each agent is only based on his private type. 
%	Thus if both agents with type $\type_1$ do not invest, the welfare for type profile $(\type_1,\type_1)$ is 0, which is strictly smaller than the benchmark. 
%	Therefore, no mechanism can help attain the benchmark in equilibrium. 
%\end{example}
%

For the investment problem, we have obtained our PoA upper bound assuming % assumed 
that both the investment decision and the realized value type are not observed by the opponents in the auction. 
In the following example, we show that the bound no longer holds if we remove this assumption. Specifically, we show that
if either the investment decision or the realized value is revealed to the opponent, there exists Nash equilibria that leads to large price of anarchy, even in the first-price auction which is a smooth mechanism.

\begin{example}\label{exp:reveal info large poa}
There are two agents and ex ante, both agents have no private information. 
Let $v>2$ be a sufficiently large constant. 
Any agent that chooses not to invest has value of 0.
If agent $1$ invests she bears a cost of $2$ and has value of $v+2$, while if agent $2$ invests she bears a cost of $v-2$ and has value of $v-1$. The optimal welfare in this setting is $v$.
%OLD: Agent 1 can choose to not invest with value $0$,  or invest with value $v$ and cost $2$.  Agent 2 can choose to not invest with value $0$, or invest with value $v-1$ and cost $v-2$. The optimal welfare in this setting is $v-2$.

Now we construct an equilibrium with large price of anarchy. 
On the equilibrium path, agent 1 does not invest, and agent 2 invests. 
Both agents bid $0$ and the item is allocated to agent 2. 
The equilibrium welfare is $1$, and the price of anarchy is at least $v$, %MB: to make this at least v, and not v-2, I have changed the value slightly 
which is unbounded when $v\to\infty$. 
Note that the above strategies can be sustained under Nash equilibrium
with the following off-path strategies. 
If agent 1 deviates to invest before the auction, 
agent 2 will observe the deviation through information from either the action or the realized valuation of agent 1, 
and then agent 2 will bid $v+2$ in the auction. 
\end{example}

Note that the above example illustrates that price of anarchy may be large even when the seller adopts a smooth auction. 
It is an interesting open question to see whether the welfare loss is small if we impose additional equilibrium refinements such as subgame perfection.
