# Supplementary material for: Making Auctions Robust to Aftermarkets
Source: arXiv:2107.05853 source file (2022-11-16)
Supplement: Supplementary file 2 [file pos.tex]

\section{Price of Stability}
\label{sec:pos}

%\mbc{minor edits below}

In this section, we analyze the price of stability result in the combined market. 
First, we made the following assumption on the secondary market $\mechs$. 

\begin{assumption}\label{asp:opt out}
For any initial allocation $\alloc$, there exists an action profile $\hat{\action}\second =\hat{\action}\second_{\alloc}\in \actions\second$ such that for any agent $i$ and any action $\action\second_i$ we have 
\begin{align*}
u_i(\mechs(\action\second_i, \hat{\action}\second_{-i}, \alloc); \type_i)
\leq u_i(\mechs(\hat{\action}\second, \alloc); \type_i)
= u_i(\alloc; \type_i).
\end{align*}
\end{assumption}
%\mbc{is this assumption related to ex-post IR? implied by it? If so, maybe replace by it.}

This assumptions implies that for every initial allocation $\alloc$ in the secondary market, 
there is a profile of actions (playing $\hat{\action}\second$) that corresponds to all agents opting out of the secondary market (so utility is the same as at the end of the auction) which is a Nash equilibrium. 
\begin{observation}\label{thm:pos}
For any signaling protocol $\Gamma$ and any mechanism $\mechs$ satisfying \Cref{asp:opt out}, 
consider the combined market $\combinedGame$.
%
%mechanism $\mechc = (\mechf, \mechs)$
%with $\mechs$ satisfying \Cref{asp:opt out},
For any family of distributions $\dists$,
we have 
\begin{align*}
\pos(\mechc, \dists) \leq \pos(\mechf, \dists). 
\end{align*}
\end{observation}
\begin{proof}
For any allocation $\alloc$, let $\hat{\action}\second_{\alloc}$ be the action profile that satisfies \Cref{asp:opt out} in the secondary market. 
For any distribution $\dist\in \dists$ and BNE strategy profile $\strategy\first\in \BNE(\dist, \mechf)$, 
let $\strategy\combined$ be the strategy profile in the combined market that 
follows strategy $\strategy\first$ in the first market,
and always chooses action profile $\hat{\action}\second_{\alloc}$
in the secondary market given allocation $\alloc$, 
regardless of the payment and the signals realized in the auction. 
%$\strategy\second$ be the strategy that always chooses action profile $\hat{\action}\second_{\alloc}$ for all types given that the initial allocation in the secondary market is $\alloc$. 
It is easy to verify that since $\hat{\action}\second_{\alloc}$ is a Nash equilibrium profile in the secondary market for any outcomes realized in the auction, 
%for any belief updated from strategy profile with full support that is a small perturbation from the equilibrium strategies, 
there is no profitable deviation strategy for any player $i$ in the combined market, 
%Thus strategy $\strategy\combined$ is sequentially rational,
i.e.,  $\strategy\combined \in \BNE(\dist,\mechc)$.
Moreover, the expected welfare given strategy $\strategy\combined$ in combined market $\mechc$
equals the expected welfare given strategy profile $\strategy\first$ in first market $\mechf$.
Therefore, the price of stability does not increase. 
\end{proof}

Note that the observation considers price of stability for BNE. It leaves open the possibility that price of stability of the combined market is higher than the price of stability of the auction for refinements of BNE and other solution concepts. 

%any information they receive in the secondary market. 
%Therefore, $\strategy\combined = \strategy\first\times\strategy\second \in \SPE(\dist,\mechc)$, 
%and the expected welfare given strategy $\strategy\combined$ in combined market $\mechc$
%equals the expected welfare given strategy $\strategy\first$ in first market $\mechf$.
