# Supplementary material for: Making Auctions Robust to Aftermarkets
Source: arXiv:2107.05853 source file (2022-11-16)
Supplement: Supplementary file 3 [file refinement.tex]

\section{Price of Anarchy under Equilibrium Refinement}
\label{apx:refine}
\begin{theorem}
For single-item setting, if the winner posts a take-or-leave-it offer to the other agent in the secondary market 
and no information is revealed in the secondary market,
under the refinement of iterative elimination of weakly dominated strategies, 
all Bayesian Nash equilibria in the combined market for the second price auction are efficient.  
\end{theorem}
\begin{proof}
For any agent~$i$, let $p_i$ be the price agent $i$ charges when she resells the item under equilibria. 
Since agent $i$ also maximizes her utility in the secondary market,
we have $\val_i\leq p_i$. 
Next we claim that any bid $b_i > p_i$
in the first stage
is weakly dominated by bidding $p_i$ 
and reselling the item with price $p_i$ in the secondary market. 
Since no information is revealed in the secondary market,
the only difference for agent $i$
is the case that the highest bid of the opponents in the auction is in the range of $(p_i,b_i)$.
In that case, she strictly benefits from lowering the bid and not winning the item since her value is $\val_i\leq p_i$.

Conditional on the event that for all agents, 
the bids in the auction are weakly lower than their price charged for reselling the item 
in the secondary market, 
it is a weakly dominant strategy for all agents to bid their value in the auction, 
since all agents get weakly higher utility for winning in the auction than in the secondary market. 
Thus the allocation is efficient in the auction, 
and no trade happens in the secondary market. 
All equilibria are efficient in the combined market. 
\end{proof}

% \begin{theorem}
% For single-item setting, given any secondary market satisfying voluntary participation and weak budget balance
% where bids are not revealed, 
% under the refinement of iterative elimination of weakly dominated strategies, 
% all equilibria in second price auction are efficient.  
% \end{theorem}
% \begin{proof}
% For any agent~$i$, let $p_i$ be the expected payment to agent $i$ when she resells the item. 
% Since the secondary market satisfies voluntary participation,
% we have $\val_i\leq p_i$. 
% Next we claim that any bid $b_i > p_i$
% in the auction environment 
% is weakly dominated by bidding $p_i$ in the auction environment and reselling the item with expected payment $p_i$ in the secondary market. 
% Note that the only difference for agent $i$
% is the case that the highest bid of the opponents in the auction is in the range of $(p_i,b_i)$.
% In that case, she strictly benefits from lowering the bid and not winning the item since her value is $\val_i\leq p_i$.

% Conditional on the event that for all agents, 
% the bids in the auction are weakly lower than their price charged for reselling the item 
% in the secondary market, 
% it is a weakly dominant strategy for all agents to bid their value in the auction, 
% since all agents get weakly higher utility for winning in the auction than in the secondary market. 
% Thus the allocation is efficient in the auction, 
% and no trade happens in the secondary market. 
% All equilibria are efficient in the combined market. 
% \end{proof}
