# Supplementary material for: Making Auctions Robust to Aftermarkets
Source: arXiv:2107.05853 source file (2022-11-16)
Supplement: Supplementary file 4 [file revenue.tex]

\section{Price of Anarchy for Revenue}
\label{sec:revenue}
In the single-item setting, 
\citet{hartline2014price} showed that 
 % when there is no secondary market, 
the first-price auction (and the  all-pay auction) with monopoly reserve
guarantees constant approximation to the optimal revenue. 
However, their result is for stand alone auctions, and their technique does not extend to the setting 
when there are secondary markets.
The main reason is that their analysis requires that agents with value below the reserve price will never get % not win 
the item, 
which is not guaranteed in our setting since for some realizations of the valuation profile,
agents may buy the item in the secondary market even if their value is below the reserve price in the auction (see \cref{exp:not sale} for an illustration). 
\citet{carroll2019robustly} characterized the optimal mechanisms that are robust to the format of the secondary market. 
They only considered the revenue under the best equilibrium, 
and the revenue guarantee under worst equilibrium is left as an open problem. 
We will address this question by considering the price of anarchy for revenue. 

\sloppy
Denote the expected revenue of $\mech$ given type distribution~$\dist$
and equilibrium strategy $\strategy$
by $\rev(\mech, \strategy,\dist) = \E_{\type\sim\dist}[\sum_i \pay^{\mech}_i(\strategy(\type))]$. 
The optimal revenue given distribution~$\dist$
is defined as 
$\rev(\dist) = \sup_{\mech\in \mathbb{M},\strategy\in \BNE(\dist, \mech)}\{\rev(\mech, \strategy, \dist)\}$
where $\mathbb{M}$ is the set of auction mechanisms satisfying voluntary participation.\footnote{Note that, by the revelation principle, this is equivalent to maximizing revenue over Bayesian incentive compatible 
and individual rational mechanisms.}
%and there is no secondary market.
Then the \emph{price of anarchy for revenue}  of mechanism $\mech$ within the family of distributions $\dists$ is 
\begin{align*}
\poar(\mech, \dists) = 
\sup_{\dist\in \dists} \frac{\rev(\dist)}{\inf_{\strategy\in \BNE(\dist, \mech)}\{\rev(\mech, \strategy, \dist)\}}.
\end{align*} 

In this section, we consider combined markets created by any ex-post IR trade mechanism, running after first-price auction with an optimal anonymous reserve (but with no information revealed after the auction). 
We assume that the  valuation distributions are regular and bounded.  
We show that even under the worst equilibrium of the combined market, the revenue of the auctioneer is at least a constant fraction of the optimal revenue. 
Our result holds under the standard Myerson regularity assumption: 
\begin{definition}
A distribution $\dist$ is \emph{regular} if the virtual value $\phi(\val)=\val - \frac{1-\dist(\val)}{f(\val)}$ is non-decreasing in~$\val$.
\end{definition}

\begin{theorem}\label{thm:poa revenue}
%\mbc{A new version of the theorem, with explicit independence  :}
Consider the single-item setting with buyers with independently drawn valuations, each from a regular distribution with bounded support.
Fix the auction $\mechf$ to first-price auction
%or second-price auction 
with optimally chosen anonymous reserve,\footnote{We assume that the item is sold if there is at least one bidder that bids the reserve or higher.}  
and fix any trade mechanism $\mechs$ satisfying ex post individual rationality. %secondary market $\mechs$ satisfying voluntary participation and weak budget balance. 
Consider the combined market 
$\combinedGameNoSignal$ in which bidders get no signal after the auction.\footnote{That is, no information about the bids is being revealed after the auction. All each agent knows is the allocation and her own payment.}
Then  the price of anarchy for revenue for the combined market 
is at most 2.62.
% OLD version: 
%For the single-item setting, when the valuation distributions are regular for all agents \mbc{are we assuming independence? } and when mechanism $\mechf$ is first-price auction or second-price auction with optimally chosen anonymous reserve,  the price of anarchy for revenue given the combined market  $\mechc = \mechf\times\mechs$ is at most 2.62, if the bids of the buyers are not revealed in the secondary market  and the secondary market $\mechs$ satisfies weak budget balance and voluntary participation. 
\end{theorem}

%\bjl{Rewrote the following paragraph to be slightly less accurate but easier to parse.  Double-check for accuracy.}

To prove \Cref{thm:poa revenue} we make use of a result by \citet{jin2019tight}, which shows that (in a setting without secondary markets) the best revenue achievable with an anonymous posted price is a $2.62$-approximation to the optimal revenue, for regular distributions.  As we will show in \Cref{lem:anonymous reserve}, a first-price auction with reserve price $r$ followed by a secondary market will generate at least as much revenue as posting an anonymous price $r$.
%\yl{removed ``again for regular distributions". Also changed statement of \cref{lem:anonymous reserve} since regularity is not required for the lemma. Regularity is only used for $2.62$-approximation. }  
Combining the results, we obtain that price of anarchy on revenue is at most $2.62$ and \Cref{thm:poa revenue} holds.

%the authors showed that when there are no secondary markets, 
%if the valuation distributions are regular, 
%anonymous pricing is a $2.62$-approximation to the optimal revenue. 
%Combining the results, we obtain that price of anarchy on revenue is at most $2.62$ and \Cref{thm:poa revenue} holds.

%As we will show in \Cref{lem:anonymous reserve}, 
%if the bids are not revealed in the secondary market, 
%the revenue loss of first-price auction or second price auction with anonymous reserve $r-\epsilon$ given any secondary market and equilibrium strategy 
%compared to the revenue of posting the 
%same reserve 
%price of $r$ 
%to all agents when there are no secondary markets
%is at most $\epsilon$ for any $\epsilon>0$. 
%In \citet{jin2019tight}, the authors showed that when there are no secondary markets, 
%if the valuation distributions are regular, 
%anonymous pricing is a $2.62$-approximation to the optimal revenue. 
%Combining the results, we obtain that price of anarchy on revenue is at most $2.62$ and \Cref{thm:poa revenue} holds.

\begin{restatable}{lemma}{lemrev}\label{lem:anonymous reserve}
%\mbc{A new version of the lemma :}
Consider the single-item setting with buyers with independently drawn valuations with bounded support.
Fix the auction $\mechf$ to be first-price auction with anonymous reserve $r$, %\mbc{added footnote.}\footnote{We assume that the item is sold if there is at least one bidder that bids the reserve or higher. } 
and fix any trade mechanism $\mechs$ satisfying ex post individual rationality. %secondary market $\mechs$ satisfying voluntary participation and weak budget balance. 
Consider the combined market 
$\combinedGameNoSignal$
in which bidders get no signal after the auction.
Then in any BNE of $\mechc$, in 
any realization of the valuations except a set with measure 0,
if there exists an agent with value strictly 
%\mbc{can we make this "weakly"? don't we need the stronger claim to prove the theorem?} \yl{This lemma requires strictly. Our theorem holds with this strict version since for approximation ratio of anonymous pricing, it doesn't matter the agent buys with weakly higher value or strictly higher value.} \mbc{Say agents have value 1 for sure. By this lemma, setting a reserve of 1 will not give any revenue guarantee. I do see that this can be solved by setting the reserve to $1-\varepsilon$ though.} 
above the reserve price $r$, 
the item is sold to some agent in the auction with probability $1$. 
% OLD: For the single-item setting, and for first-price auction or second-price auction with anonymous reserve,  if the bids of the buyers are not revealed in the secondary market  and the secondary market satisfies weak budget balance and voluntary participation,  then the item is sold if there exists an agent with value strictly above the reserve price. 
\end{restatable}
%\yl{added intuition for \cref{lem:anonymous reserve}}

Intuitively, for any agent with value strictly above the reserve price $r$, 
if her bid in the auction is below~$r$, 
then consider what would happen if she increases her bid to $r$.  There are two cases:
\begin{itemize}
\item if the item was previously not being sold at all, then the agent will win the item by raising her bid to the reserve price.%\mbc{as you know there is an issue with ties. I have added a footnote to make it clear that wlog we can assume that if someone bids exactly the reserve the item is sold. I see no problem making this assumption (as it is about the auction format, not about agent behavior - what we CANNOT assume is that an agent with value exactly $r$ bids $r$. But here it seems we assume the value is strictly more than $r$). With it, can't we simplify the proof? I am not sure the zero measure will be needed, and other things might also be easier. 
%	If we decide if this is ok, we also need to change the discussion about ties later in this section  }  
In this case, her utility in the combined market strictly increases by this deviation (since originally her utility in the combined mechanism was $0$, as the item was going unallocated).

\item if the item was previously being sold to some other agent, then the agent's utility is not impacted by this bid increase in the auction, since information on bids is not revealed in the secondary market so the auction winner cannot observe this deviation.
%and the winner in the auction cannot observe this deviation. 
%Her utility remains the in this case in the combined market.
\end{itemize}

We conclude that in order for an agent to bid below~$r$ at equilibrium, 
it must be that the first case occurs with probability $0$. 
This means that the item is always sold, as claimed by \cref{lem:anonymous reserve}.
This intuitive argument does not account carefully for tie-breaking between bids, which is important since the proposed deviation involves bids that are equal to the reserve price. The formal proof is provided at the end of the section
with additional careful analysis of the tie-breakings in the auction.

Note that in \Cref{lem:anonymous reserve}, it is crucial to assume that the bids are not revealed in the secondary market. 
This is a natural assumption if the mechanism designer has control over the bid information and chooses not the reveal such information to the secondary market. 
The following example illustrate the failure of \Cref{lem:anonymous reserve} if bids are revealed. 
\begin{example}\label{exp:not sale}
Consider there are $3$ agents. 
\begin{itemize}
\item Agent $1$ has value $1.1$.
\item Agent $2$ has value $0$ with probability $\frac{3}{4}$
and value $2$ with probability $\frac{1}{4}$.
\item Agent $3$ has value $0$ with probability $\frac{1}{4}$
and value $10$ with probability $\frac{3}{4}$.
\end{itemize}
Suppose the auctioneer chooses first-price auction with reserve price $1$. 
Now consider the specific secondary market where 
if the bid profile in auction is $(0,2,1)$,
then agent $2$ has the option to sell the item to agent $3$, 
and if there is a sale then  agent $2$ receives a payment of $3$ 
and agent $3$ pays $4$ for the item, and  
%\mbc{this is not strongly BB, so it is a little strange and the reader might suspect it is the reason for the failure of \Cref{lem:anonymous reserve}. Is it the case ? Can we change the example to satisfy strong BB?} 
additionally,  if the trade happens then agent $1$ also receives a payment of $1$ (making the mechanism strongly budget balanced.) 
If the bid profile in auction is not $(0,2,1)$, 
no trade can occur in the secondary market.

It is easy to verify that in this setting, 
the following is a Bayesian Nash equilibrium strategy for all agents. 
Agent $1$ bids $0$, 
agent $2$ bids $2$ if her value is $2$ and $0$ otherwise, 
and agent $3$ bids $1$ if her value is $10$ and $0$ otherwise.
Moreover, under this equilibrium, the item is not sold if both agent $2$ and agent $3$ has value $0$, which occurs with probability $\frac{3}{16}$,
%and the revenue of the mechanism is only $\frac{3}{4}$
even though agent $1$ has value strictly above reserve price $1$ with probability~$1$. 
\end{example}

% \section{Missing Proofs from Section \ref{sec:revenue}}
% \label{apx:proof revenue}

%\begin{numberedlemma}{\ref{lem:anonymous reserve} (restated)}
%Consider the single-item setting with buyers with independently drawn valuations, each from a regular distribution with finite support.
%Fix the auction $\mechf$ to be first-price auction with anonymous reserve $r$, 
%and fix any trade mechanism $\mechs$ satisfying ex post individual rationality. %secondary market $\mechs$ satisfying voluntary participation and weak budget balance. 
%Consider the combined market 
%$\combinedGameNoSignal$
%in which bidders get no signal after the auction.
%Then in any BNE of $\mechc$, in 
%any realization of the valuations except a set with measure 0,
%if there exists an agent with value strictly 
%above the reserve price $r$, the item is sold to some agent in the auction. 
%\end{numberedlemma}
% \lemrev*
\begin{proof}[Proof of \cref{lem:anonymous reserve}] 
If the measure of profiles of agents types such that for some agent $i$ it holds that 
$v_i > r$ and $b_i(v_i) < r$ is 0, \cref{lem:anonymous reserve} clearly holds.
Assume that this measure is positive.  
%OLD: If the measure of agents with value  $v_i > r$ and $b_i(v_i) < r$ is 0,  \cref{lem:anonymous reserve} holds. 
%Now suppose that the set of agents with value  $v_i > r$ and $b_i(v_i) < r$ has strictly positive measure. 
We show that in this case, the item is sold with probability 1. 
%For each agent $i \in I$, let $\bar{v}_i$ be the supreme value such that 
%$b_i(\bar{v}_i) < r$. 
%For each agent $i\not\in I$, let $\bar{v}_i = r$.

Let $H<\infty$ be larger than the highest value of the support of any agent. % Moved to here, no need for it to be above.
Let $\event$ be the event such that the highest bid among all agents is $r$.
First we consider the case that the probability of event $\event$ is strictly positive, 
and denote the probability by~$p$. 
\begin{claim}
Conditional on event~$\event$, 
for any agent $i$ with value $\val_i > r$ and equilibrium bid $b_i(v_i) = r$, 
if agent~$i$ loses in the auction with positive probability $p'>0$
then the  expected per-unit price (expected payment divided by expected allocation) 
for purchasing the item in the secondary market is at most $r$.
\end{claim}
\begin{proof}
Assume by contradiction that the per-unit price paid by agent $i$ is $r+\epsilon$ for some constant $\epsilon>0$. 
Let $\epsilon' < \frac{\epsilon p\cdot p'}{4}$ be the number such that $r+\epsilon' < v_i$
and the probability the highest bid between $(r, r+\epsilon']$ is at most $\frac{\epsilon p\cdot p'}{4H}$. 
Note that for agent~$i$,
one possible deviation strategy is to bid $r+\epsilon'$ in the auction, 
and follow the equilibrium strategy in the secondary market.  To analyze the utility obtained under such a deviation, consider cases for the highest competing bid in the auction.

%\bjl{Changed some $\epsilon$ to $\epsilon'$ -- check that it is correct.  I also explicitly rewrote this as a case analysis.}

\begin{itemize}
\item Case 1: $\max_{j\neq i} b_j > r+\epsilon'$.  In this case agent $i$ does not win the item,
and since the bid of agent $i$ is not revealed, 
the utility of agent $i$ remains the same. 

\item Case 2: $\max_{j\neq i} b_j \in (r, r+\epsilon']$.
The probability of this case is at most $\frac{\epsilon p\cdot p'}{4H}$, 
and hence the maximum possible expected utility loss that agent $i$ can experience due to this case is at most $\frac{\epsilon p\cdot p'}{4}$.

\item Case 3: $\max_{j\neq i} b_j < r$.  In this case agent $i$ will win the item with a bid of $r + \epsilon'$.
%If agent $i$'s equilibrium bid smaller than $r$, 
%then the utility of agent $i$ increases by winning the item with bid $r+\epsilon'$.
This can lead to a utility loss only if, at equilibrium, agent $i$ is bidding exactly $r$ and winning the item.
%If under equilibrium agent $i$ bids $r$,
In this case the utility of agent $i$ decreases by $\epsilon'$, since his bid increases by $\epsilon'$.
The expected utility loss due to this case is therefore at most $\epsilon'\leq \frac{\epsilon p\cdot p'}{4}$.

\item Case 4: $\max_{j\neq i} b_j = r$.
In this case agent $i$ will win the item.
If at equilibrium agent $i$ bids $r$ and wins, 
then the utility of agent $i$ decreases by $\epsilon'\leq \frac{\epsilon p\cdot p'}{4}$.
If under equilibrium agent $i$ loses (either with a bid of $r$ or strictly less than $r$), which happens with probability at least $p\cdot p'$, 
then the utility of agent $i$ is increased by $\epsilon - \epsilon' > \frac{3\epsilon}{4H}$
since originally agent $i$ pays $r+\epsilon$ per-unit price (in the secondary market), 
while currently the agent $i$ wins with payment $r+\epsilon'$
and the resale will not decrease the utility of agent $i$.
Thus the expected utility increase due to this case is strictly larger than $\frac{3\epsilon p\cdot p'}{4}$.
\end{itemize}

Combining all these cases, we note that total expected utility increases under this deviation for agent~$i$, which contradicts to the assumption that bidding at most $r$ is an equilibrium strategy. 
We conclude that for any agent $i$ with value $v_i > r$ and bid $b_i(v_i) \leq r$, who loses in the auction with positive probability, the expected per-unit price in the secondary market is at most $r$.
\end{proof}

%\mbc{Isn't the next paragraph part of the proof of the claim?}
%\yl{No this mainly proving the following bold sentence.}
%\mbc{so I think it is better to encapsulate it in a claim. It should be the case that  the reader can fully understand the proof of the lemma from the statements of the claims and the text combining them (without reading the proof of each claim). This should also be the case for the proof in Appendix C. }

On the other hand, for any agent with 
$v_i\leq r$, the expected per-unit price paid by agent $i$ in the secondary market conditional on losing in the auction is at most $r$
given any valuation profile of other agents, 
since the secondary market satisfies ex post individual rationality. 
This implies the following claim. 
\begin{claim}\label{clm4}
For any agent $i$ with value $\val_i > r$ and equilibrium bid $b_i(v_i) < r$, 
except for a set of measure~0,
the per-unit price paid by agent~$i$ in the secondary market is at least~$r$ conditional on event~$\event$. 
\end{claim}
\begin{proof}
To see why this is true, suppose otherwise.  Then conditional on event $\event$ happening, 
for any agent $j$ not winning the auction, 
the bid of agent~$j$ is at most $r$, and the per-unit price paid by agent $j$ is at most~$r$. 
This implies that the average per-unit price paid by agents losing in the auction is strictly less than $r$.
Thus there exists an agent $j^*$ with value $\val_{j^*}$
and bid $\bid_{j^*}(\val_{j^*})=r$ winning the auction
such that the expected per-unit price for reselling the item in the secondary market is strictly below~$r$ conditional on agent $j$ winning the item. 
If $\val_j \geq r$, this implies that the secondary market does not satisfy voluntary participation for agent $j$, 
and if $\val< r$, the utility of agent~$j$ is negative in the combined market, 
and agent~$j$ can deviate to bid $0$ in the auction to retain utility $0$, 
which violates the assumption of the equilibrium.  So in either case we arrive at a contradiction, and hence the claim follows.
\end{proof}

%First we claim that there exists an agent $i^*\in I$ with value $\bar{\val}_{i^*}$ 
%such that conditional on the highest bid in the auction being $r$,
%the expected per-unit price (expected payment divided by expected allocation) 
%for purchasing the item in the secondary market is at least $r$.
%This holds because otherwise there exists an agent $j$ with value $\val_j$
%and bid $\bid_j(\val_j)=r$ 
%such that the expected per-unit price for reselling the item in the secondary market is below~$r$ conditional on winning the item. 
%If $\val_j \geq r$, this implies that the secondary market does not satisfy voluntary participation for agent $j$, 
%and if $\val< r$, the utility of agent~$j$ is negative in the combined market, 
%and agent~$j$ can deviate to bid $0$ in the auction to retain utility $0$, 
%which violates the assumption of the equilibrium.

Note that since we assumed the measure of profiles of agents types such that for some agent $i$ it holds that 
$v_i > r$ and $b_i(v_i) < r$ is strictly positive,
\cref{clm4} implies that 
there exists an agent $i^*$ such that $v_i>r$, $b_i(v_i)<r$, and the per-unit price paid by agent~$i^*$ conditional on event $\event$ is at least $r$.

\begin{claim}\label{clm:prob1}
If event $\event$ happens with positive probability, 
if there exists an agent $i^*$ such that $v_i>r$, $b_i(v_i)<r$, and the per-unit price paid by agent~$i^*$ conditional on event $\event$ is at least $r$, 
then the item is sold with probability 1.
\end{claim}
\begin{proof}
One possible deviation strategy for agent $i^*$ is to bid $r$ in the auction, 
and follow the equilibrium strategy in the secondary market. 
We consider three different cases for the bid of other agents. 
\begin{enumerate}
\item Suppose $\max_{j\neq i^*} b_j < r$. In this case, the item is not sold to any agent, 
which implies that agent $i^*$ strictly benefits from deviating to bid $r$ and win the item with price $r$
since $b_{i^*} - r > 0$. 

\item Consider the case where $\max_{j\neq i^*} b_j \geq r$ and the item is sold to agent $j^*\neq i^*$ even if agent $i^*$ has bid $r$. 
For agent $i^*$, by deviating the bid to $r$, 
the allocations and payments of the auction are not affected, 
and since the bids are not revealed in the secondary market, 
the utility of agent $i^*$ remains the same in the combined market.

\item Consider the case where $\max_{j\neq i^*} b_j = r$, i.e., conditional on event $\event$,
and when agent~$i^*$ deviate the bid to $r$, she wins the item.
By the definition of $i^*$, 
the per-unit price paid to other agents for reselling the item in the secondary market is at least $r$, 
which implies that the utility of agent~$i^*$ in the combined market is at most $\val_{i^*} - r$. 
Moreover, by bidding $r$ and winning the item, 
the utility of agent $i^*$ is at least $\val_{i^*} - r$. 
\end{enumerate}
Combining these cases, we conclude that for agent $i^*$ with value $\val_{i^*} > r$, 
the utility for bidding $r$ is weakly higher than the utility for bidding strictly below $r$. 
Moreover, the equality holds only when the probability of case 1 is 0,
which implies that the item is sold with probability~1. 
\end{proof}

Finally consider the case that event $\event$ happens with probability $0$.
In this case for any agent $i$ with value $\val_i > r$, 
the utility for bidding $r$ is weakly higher than the utility for bidding strictly below $r$
since the third case discussed in \cref{clm:prob1} happens with probability~$0$. 
Moreover, the equality holds only when the probability of case 1 is 0,
which implies that the item is sold with probability~1.
\end{proof}

%Finally, next example provides justifications for only comparing to the optimal revenue without secondary market
%in the definition of price of anarchy for revenue. 
%\begin{example}\label{exp:large rev}
%Suppose there are two agents. Agent 1 has value 1 and agent 2 has valuation distribution $F(\val) = 1-\frac{1}{\val}$ for any $\val \in [1,H)$ and $F(H)=1$. 
%The optimal revenue for the combined market is $\log H$ 
%if the secondary market satisfies that the valuations are public information and agent 1 has full bargaining power.
%This is obtained by selling the item to agent 1 with price $\log H$, 
%and agent 1 resales the item to agent 2 with price $\val$.
%In contrast, for any auction mechanism, the worst case revenue over the all possible secondary markets 
%is at most the optimal revenue when is no secondary markets, 
%which is at most 1. 
%The gap is unbounded when $H\to \infty$.
%\end{example}
