# Supplementary material for: Making Auctions Robust to Aftermarkets
Source: arXiv:2107.05853 source file (2022-11-16)
Supplement: Supplementary file 5 [file single.tex]

\section{Efficiency for Single Strategic Agent}

\mbc{If we keep this section we need to point to it in the intro.}
\yl{I actually prefer removing this since it seems that this does not fit well with the rest of the story.}

In this section, we consider the special case of selling a divisible item to a group of agents where there is only a single strategic agent. 
We assume that all other agents are price taker and the demand of those agents are infinitesimal. 
The strategic agent is ignorant of the individual valuation function of other agents but aware of the aggregated valuation function. 
The benefit of studying this model is to characterize the behavior of the agent in the combined market without worrying about the equilibrium selection in the secondary market. 
Let $v_1(q)$ be the value of the strategic agent for quantity $q$ 
and $v_2(q)$ be the aggregated welfare of the rest of the agents.
\begin{definition}
An agent $i$ has \emph{continuous non-increasing marginal valuation} if 
$v'_i(q) \geq 0, v''_i(q) \leq 0$ for any $q\in [0, 1]$. 
\end{definition}
% We assume that all agents have continuous non-increasing marginal valuation, 
% which implies that $v'_1(q) > 0, v''_1(q) < 0$ and $v'_2(q) > 0, v''_2(q) < 0$.
% We show that under this assumption, 
% the welfare in the combined market is always weakly higher than the welfare without secondary market. 
In the auction environment, all agents simultaneously declare valuation functions. 
% and the item is sold at the market clearing price \mbc{there might be more than one clearing price. need to break ties carefully}. 
In the secondary market, 
the strategic agent offers a uniform trading price 
to the price takers, 
and those agents purchase the item from the strategic agent if the marginal value for the additional item exceeds the price, 
and sell the item if the marginal value for the item is below the price. 
% In the secondary market, 
% the strategic agent offers a uniform price to the price takers and purchase \mbc{the fact he buys from them and never sells to them is a result, not an assumption. We need to allow both options apriori} from all other agents the fraction of their allocations with marginal value below the price. 

\begin{definition}
Let $A$ and $B$ be two subsets of $\reals$. 
We say that $B$ is weakly greater than $A$ according to the strong set order (denoted by $B \geq A$) if for any $a \in A$ and $b \in B$, if $a > b$, then
$a \in B$ and $b \in A$.
\end{definition}

% \mbc{The theorem below seems to be missing the solution concept. 
% Here we need to add something like "In the next theorem the "social welfare of a market"
% is the set of all possible welfare values obtained when considering all subgame perfect equilibria of that market." (and maybe also discuss undominated strategies - I think they might not be needed here.)}

\mbc{the statement of this theorem need to be revised to be explicit about the setting, assumptions about information ad $\mechs$ etc., like all other thorems in the body.   }
\begin{theorem}\label{thm:strong set order}
If all agents have continuous non-increasing marginal valuations, 
when the price-takers bid truthfully 
and the strategic agent best responses, 
the social welfare in the combined market is weakly greater than the welfare without secondary market in strong set order.
\end{theorem}
\begin{proof}
First note that if the strategic agent 
enters the secondary market with endowment $q_0$,
% acquired $q_0$ fraction of the item in the auction, 
% in the secondary market, 
his utility in the secondary market 
is $u_1(q, q_0)=v_1(q)-v'_2(1-q)(q-q_0)$
if he receives a total of $q$ fraction of the items when he posts price $p = v'_2(1-q)$. 
Thus the optimal price $p^*$ in the secondary market satisfies
\begin{enumerate}
    \item $v'_2(1-q^*) = p^*$;
    \item $q^* = \argmax_q u_1(q, q_0)$.
\end{enumerate}
Since the utility function $u_1(q, q_0)$ is supermodular in $q$ and $q_0$. 
Note that the optimal choice $q^*$ may not be unique. 
By Topkis's Theorem, 
$q^*(q_0)$ is monotone increasing in $q_0$ in strong set order. 
Moreover, if $q_0 = 0$, the resulting allocation $q^*(0)$ is equivalent to the allocation of all agents participate the auction without secondary market. 
Thus in the combined market, for the optimal strategy of the strategic player, 
his allocation is greater than the case without secondary market in strong set order. 
Moreover, the marginal value of the strategic agent for quantities between $q^*(q_0)$ and $q^*(0)$ is higher than the rest of the agents. 
Hence the social welfare improves in strong set order. 
\end{proof}

A corollary to \Cref{thm:strong set order} is that,
if the optimal choice of the strategic agent is unique in the auction without secondary market, 
then the optimal welfare weakly improves with the presence of the secondary market.
