# Supplementary material for: Making Auctions Robust to Aftermarkets
Source: arXiv:2107.05853 source file (2022-11-16)
Supplement: Supplementary file 6 [file subadditive.tex]

\section{Price of Anarchy for Subadditive Valuations}
\label{sec:subadditive}
In literature, there exists techniques other than the smooth framework that delivers tight bounds on the price of anarchy
in multi-item settings. 
For example, \cite{feldman2013simultaneous} showed that
for subadditive valuations, 
the price of anarchy of simultaneous first price auction is $2$ 
while the bound derive from smooth framework is only logarithmic. 
However, the ideas for bounding the the price of anarchy
is still analogous to the smooth framework, 
which is established by showing that there exists a randomized action profile for each agent with sufficiently large utility. 
Thus our reduction framework in \Cref{sec:smooth} can also be generalized for this setting. 
The result is formalized in the following theorem. 
Note that the main take away for this section is 
not simply providing a proof for the price of anarchy for subadditive valuations,
but to illustrate that the ideas in our reduction framework is broadly applicable beyond the conventional smooth framework.\footnote{\cite{syrgkanis2012bseq} show that the sequential first price auction has price of anarchy $\frac{2e}{e-1}$ for unit-demand valuation. 
Similarly, one can apply our technique in their setting and show that this result can also be generalized for any secondary market satisfying voluntary participation and weak budget balance.
The details are omitted in this paper.} 

\begin{theorem}\label{thm:subadditive}
For multi-unit setting,
given any secondary market satisfying voluntary participation and weak budget balance,
the price of anarchy of simultaneous first price auction is at most $2$ for subadditive valuations
when the prior distributions are independent.
\end{theorem}

The proof of \Cref{thm:subadditive} builds on the following two Lemmas.
\begin{lemma}[\citealp{feldman2013simultaneous}]
\label{lem:sub1}
For any agent with subadditive valuation, 
and for any distribution $D$ over prices on $m$ items, 
there exists a bid $\bid$ over $m$ items such that 
\begin{align*}
\expect[p\sim D]{\val(\bid,p)} - \sum_{j=1}^m b_j
\geq \frac{1}{2} \val([m]) - \expect[p\sim D]{\sum_{j=1}^m p_j}
\end{align*}
where $\val(\bid,p)$ is the value of the agent for bidding $\bid$ against price $p$ in the first price auction. 
\end{lemma}

\begin{lemma}[\citealp{feldman2013simultaneous}]
\label{lem:sub2}

\end{lemma}

\begin{proof}[Proof of \Cref{thm:subadditive}]

\end{proof}
