# Supplementary material for: Making Auctions Robust to Aftermarkets
Source: arXiv:2107.05853 source file (2022-11-16)
Supplement: Supplementary file 7 [file revenue.tex]

% \section{Missing Proofs from Section \ref{sec:revenue}}
% \label{apx:proof revenue}

%\begin{numberedlemma}{\ref{lem:anonymous reserve} (restated)}
%Consider the single-item setting with buyers with independently drawn valuations, each from a regular distribution with finite support.
%Fix the auction $\mechf$ to be first-price auction with anonymous reserve $r$, 
%and fix any trade mechanism $\mechs$ satisfying ex post individual rationality. %secondary market $\mechs$ satisfying voluntary participation and weak budget balance. 
%Consider the combined market 
%$\combinedGameNoSignal$
%in which bidders get no signal after the auction.
%Then in any BNE of $\mechc$, in 
%any realization of the valuations except a set with measure 0,
%if there exists an agent with value strictly 
%above the reserve price $r$, the item is sold to some agent in the auction. 
%\end{numberedlemma}
% \lemrev*
\begin{proof}[Proof of \cref{lem:anonymous reserve}] 
If the measure of profiles of agents types such that for some agent $i$ it holds that 
$v_i > r$ and $b_i(v_i) < r$ is 0, \cref{lem:anonymous reserve} clearly holds.
Assume that this measure is positive.  
%OLD: If the measure of agents with value  $v_i > r$ and $b_i(v_i) < r$ is 0,  \cref{lem:anonymous reserve} holds. 
%Now suppose that the set of agents with value  $v_i > r$ and $b_i(v_i) < r$ has strictly positive measure. 
We show that in this case, the item is sold with probability 1. 
%For each agent $i \in I$, let $\bar{v}_i$ be the supreme value such that 
%$b_i(\bar{v}_i) < r$. 
%For each agent $i\not\in I$, let $\bar{v}_i = r$.

Let $H<\infty$ be larger than the highest value of the support of any agent. % Moved to here, no need for it to be above.
Let $\event$ be the event such that the highest bid among all agents is $r$.
First we consider the case that the probability of event $\event$ is strictly positive, 
and denote the probability by~$p$. 
\begin{claim}
Conditional on event~$\event$, 
for any agent $i$ with value $\val_i > r$ and equilibrium bid $b_i(v_i) = r$, 
if agent~$i$ loses in the auction with positive probability $p'>0$
then the  expected per-unit price (expected payment divided by expected allocation) 
for purchasing the item in the secondary market is at most $r$.
\end{claim}
\begin{proof}
Assume by contradiction that the per-unit price paid by agent $i$ is $r+\epsilon$ for some constant $\epsilon>0$. 
Let $\epsilon' < \frac{\epsilon p\cdot p'}{4}$ be the number such that $r+\epsilon' < v_i$
and the probability the highest bid between $(r, r+\epsilon']$ is at most $\frac{\epsilon p\cdot p'}{4H}$. 
Note that for agent~$i$,
one possible deviation strategy is to bid $r+\epsilon'$ in the auction, 
and follow the equilibrium strategy in the secondary market.  To analyze the utility obtained under such a deviation, consider cases for the highest competing bid in the auction.

%\bjl{Changed some $\epsilon$ to $\epsilon'$ -- check that it is correct.  I also explicitly rewrote this as a case analysis.}

\begin{itemize}
\item Case 1: $\max_{j\neq i} b_j > r+\epsilon'$.  In this case agent $i$ does not win the item,
and since the bid of agent $i$ is not revealed, 
the utility of agent $i$ remains the same. 

\item Case 2: $\max_{j\neq i} b_j \in (r, r+\epsilon']$.
The probability of this case is at most $\frac{\epsilon p\cdot p'}{4H}$, 
and hence the maximum possible expected utility loss that agent $i$ can experience due to this case is at most $\frac{\epsilon p\cdot p'}{4}$.

\item Case 3: $\max_{j\neq i} b_j < r$.  In this case agent $i$ will win the item with a bid of $r + \epsilon'$.
%If agent $i$'s equilibrium bid smaller than $r$, 
%then the utility of agent $i$ increases by winning the item with bid $r+\epsilon'$.
This can lead to a utility loss only if, at equilibrium, agent $i$ is bidding exactly $r$ and winning the item.
%If under equilibrium agent $i$ bids $r$,
In this case the utility of agent $i$ decreases by $\epsilon'$, since his bid increases by $\epsilon'$.
The expected utility loss due to this case is therefore at most $\epsilon'\leq \frac{\epsilon p\cdot p'}{4}$.

\item Case 4: $\max_{j\neq i} b_j = r$.
In this case agent $i$ will win the item.
If at equilibrium agent $i$ bids $r$ and wins, 
then the utility of agent $i$ decreases by $\epsilon'\leq \frac{\epsilon p\cdot p'}{4}$.
If under equilibrium agent $i$ loses (either with a bid of $r$ or strictly less than $r$), which happens with probability at least $p\cdot p'$, 
then the utility of agent $i$ is increased by $\epsilon - \epsilon' > \frac{3\epsilon}{4H}$
since originally agent $i$ pays $r+\epsilon$ per-unit price (in the secondary market), 
while currently the agent $i$ wins with payment $r+\epsilon'$
and the resale will not decrease the utility of agent $i$.
Thus the expected utility increase due to this case is strictly larger than $\frac{3\epsilon p\cdot p'}{4}$.
\end{itemize}

Combining all these cases, we note that total expected utility increases under this deviation for agent~$i$, which contradicts to the assumption that bidding at most $r$ is an equilibrium strategy. 
We conclude that for any agent $i$ with value $v_i > r$ and bid $b_i(v_i) \leq r$, who loses in the auction with positive probability, the expected per-unit price in the secondary market is at most $r$.
\end{proof}

%\mbc{Isn't the next paragraph part of the proof of the claim?}
%\yl{No this mainly proving the following bold sentence.}
%\mbc{so I think it is better to encapsulate it in a claim. It should be the case that  the reader can fully understand the proof of the lemma from the statements of the claims and the text combining them (without reading the proof of each claim). This should also be the case for the proof in Appendix C. }

On the other hand, for any agent with 
$v_i\leq r$, the expected per-unit price paid by agent $i$ in the secondary market conditional on losing in the auction is at most $r$
given any valuation profile of other agents, 
since the secondary market satisfies ex post individual rationality. 
This implies the following claim. 
\begin{claim}\label{clm4}
For any agent $i$ with value $\val_i > r$ and equilibrium bid $b_i(v_i) < r$, 
except for a set of measure~0,
the per-unit price paid by agent~$i$ in the secondary market is at least~$r$ conditional on event~$\event$. 
\end{claim}
\begin{proof}
To see why this is true, suppose otherwise.  Then conditional on event $\event$ happening, 
for any agent $j$ not winning the auction, 
the bid of agent~$j$ is at most $r$, and the per-unit price paid by agent $j$ is at most~$r$. 
This implies that the average per-unit price paid by agents losing in the auction is strictly less than $r$.
Thus there exists an agent $j^*$ with value $\val_{j^*}$
and bid $\bid_{j^*}(\val_{j^*})=r$ winning the auction
such that the expected per-unit price for reselling the item in the secondary market is strictly below~$r$ conditional on agent $j$ winning the item. 
If $\val_j \geq r$, this implies that the secondary market does not satisfy voluntary participation for agent $j$, 
and if $\val< r$, the utility of agent~$j$ is negative in the combined market, 
and agent~$j$ can deviate to bid $0$ in the auction to retain utility $0$, 
which violates the assumption of the equilibrium.  So in either case we arrive at a contradiction, and hence the claim follows.
\end{proof}

%First we claim that there exists an agent $i^*\in I$ with value $\bar{\val}_{i^*}$ 
%such that conditional on the highest bid in the auction being $r$,
%the expected per-unit price (expected payment divided by expected allocation) 
%for purchasing the item in the secondary market is at least $r$.
%This holds because otherwise there exists an agent $j$ with value $\val_j$
%and bid $\bid_j(\val_j)=r$ 
%such that the expected per-unit price for reselling the item in the secondary market is below~$r$ conditional on winning the item. 
%If $\val_j \geq r$, this implies that the secondary market does not satisfy voluntary participation for agent $j$, 
%and if $\val< r$, the utility of agent~$j$ is negative in the combined market, 
%and agent~$j$ can deviate to bid $0$ in the auction to retain utility $0$, 
%which violates the assumption of the equilibrium.

Note that since we assumed the measure of profiles of agents types such that for some agent $i$ it holds that 
$v_i > r$ and $b_i(v_i) < r$ is strictly positive,
\cref{clm4} implies that 
there exists an agent $i^*$ such that $v_i>r$, $b_i(v_i)<r$, and the per-unit price paid by agent~$i^*$ conditional on event $\event$ is at least $r$.

\begin{claim}\label{clm:prob1}
If event $\event$ happens with positive probability, 
if there exists an agent $i^*$ such that $v_i>r$, $b_i(v_i)<r$, and the per-unit price paid by agent~$i^*$ conditional on event $\event$ is at least $r$, 
then the item is sold with probability 1.
\end{claim}
\begin{proof}
One possible deviation strategy for agent $i^*$ is to bid $r$ in the auction, 
and follow the equilibrium strategy in the secondary market. 
We consider three different cases for the bid of other agents. 
\begin{enumerate}
\item Suppose $\max_{j\neq i^*} b_j < r$. In this case, the item is not sold to any agent, 
which implies that agent $i^*$ strictly benefits from deviating to bid $r$ and win the item with price $r$
since $b_{i^*} - r > 0$. 

\item Consider the case where $\max_{j\neq i^*} b_j \geq r$ and the item is sold to agent $j^*\neq i^*$ even if agent $i^*$ has bid $r$. 
For agent $i^*$, by deviating the bid to $r$, 
the allocations and payments of the auction are not affected, 
and since the bids are not revealed in the secondary market, 
the utility of agent $i^*$ remains the same in the combined market.

\item Consider the case where $\max_{j\neq i^*} b_j = r$, i.e., conditional on event $\event$,
and when agent~$i^*$ deviate the bid to $r$, she wins the item.
By the definition of $i^*$, 
the per-unit price paid to other agents for reselling the item in the secondary market is at least $r$, 
which implies that the utility of agent~$i^*$ in the combined market is at most $\val_{i^*} - r$. 
Moreover, by bidding $r$ and winning the item, 
the utility of agent $i^*$ is at least $\val_{i^*} - r$. 
\end{enumerate}
Combining these cases, we conclude that for agent $i^*$ with value $\val_{i^*} > r$, 
the utility for bidding $r$ is weakly higher than the utility for bidding strictly below $r$. 
Moreover, the equality holds only when the probability of case 1 is 0,
which implies that the item is sold with probability~1. 
\end{proof}

Finally consider the case that event $\event$ happens with probability $0$.
In this case for any agent $i$ with value $\val_i > r$, 
the utility for bidding $r$ is weakly higher than the utility for bidding strictly below $r$
since the third case discussed in \cref{clm:prob1} happens with probability~$0$. 
Moreover, the equality holds only when the probability of case 1 is 0,
which implies that the item is sold with probability~1.
\end{proof}
