# Supplementary material for: Making Auctions Robust to Aftermarkets
Source: arXiv:2107.05853 source file (2022-11-16)
Supplement: Supplementary file 10 [file additional_example.tex]

\section{Additional Example}
\label{apx:additional example}
